# Supplementary material for: PrismaCoder: Pushing the Boundaries of Open Multimodal Code Intelligence through Decomposed Rubric Synthesis
Source: arXiv:2610.20538 source file (2026-10-14)
Supplement: Supplementary file 3 [file artifactsbench.tex]

\setlength{\tabcolsep}{3pt}
\caption{ArtifactsBench, overall and per-domain scores. }
\label{tab:artifactsbench-full}
\begin{tabular}{l c ccccc}
\toprule
Model & Overall
& \makecell{Game\\Dev.} & \makecell{SVG\\Gen.} & \makecell{Web\\Apps} & \makecell{Simu-\\lation} & \makecell{Mgmt.\\Sys.} \\
\midrule
\multicolumn{7}{l}{\textit{Open models}} \\
JanusCoderV-7B & 31.16 & 27.95 & 28.97 & 33.32 & 34.04 & 33.64 \\
VinciCoder-7B  & 11.35 & 10.51 & 12.04 & 12.48 & 11.48 & 11.29 \\
VinciCoder-8B  & 11.97 & 11.06 & 14.94 & 12.34 & 11.27 & 12.10 \\
VisCoder2  & 17.51 & 16.49 & 20.43 & 18.46 & 18.13 & 15.98 \\
\rowcolor{boxblue} \textbf{\modelnine} & 45.28 & 44.49 & 50.95 & 46.22 & 48.23 & 42.27 \\
\rowcolor{boxblue} \textbf{\modelthirtyfive} & 46.01 & 54.33 & 45.00 & 44.51 & 58.53 & 37.09 \\
\midrule
\multicolumn{7}{l}{\textit{Proprietary}} \\
\rowcolor[gray]{0.92} \gptfouro & 33.54 & 36.96 & 39.54 & 39.27 & 35.73 & 35.83 \\
\bottomrule
\end{tabular}
