# Supplementary material for: PrismaCoder: Pushing the Boundaries of Open Multimodal Code Intelligence through Decomposed Rubric Synthesis
Source: arXiv:2610.20538 source file (2026-10-14)
Supplement: Supplementary file 5 [file chartmimic.tex]

\setlength{\tabcolsep}{3pt}
\caption{ChartMimic, full metrics for the Direct-1800 splits.}
\label{tab:chartmimic-full}

\begin{tabular}{l cccccccc}
\toprule
& \multicolumn{8}{c}{Direct} \\
\cmidrule(lr){2-9}
Model
& \makecell{Exec.\\Rate}
& Text
& Layout
& Type
& Color
& \makecell{Avg.\\(L)}
& \makecell{GPT\\(H)}
& Overall \\
\midrule

\multicolumn{9}{l}{\textit{Open models}} \\

JanusCoder-7B
& 89.16 & 77.61 & 85.49 & 70.06 & 67.34 & 75.12 & 68.97 & 72.05 \\

JanusCoder-8B
& 80.91 & 73.10 & 81.19 & 65.00 & 69.03 & 76.54 & 69.23 & 72.89 \\

VinciCoder-7B
& 90.88 & 79.91 & 87.99 & 73.72 & 71.59 & 78.30 & 66.09 & 72.20 \\

VinciCoder-8B
& 90.72 & 79.78 & 86.62 & 73.03 & 70.95 & 77.59 & 66.44 & 72.01 \\

\rowcolor{boxblue}
\textbf{\modelnine}
& 95.50
& 88.78
& 92.77
& 74.87
& 69.88
& 81.57
& 73.82
& 77.70 \\

\rowcolor{boxblue}
\textbf{\modelthirtyfive}
& \textbf{96.16}
& \textbf{90.41}
& \textbf{94.00}
& \textbf{76.28}
& \textbf{73.01}
& \textbf{83.42}
& \textbf{80.69}
& \textbf{82.05} \\

\midrule
\multicolumn{9}{l}{\textit{Proprietary}} \\

\rowcolor[gray]{0.92}
\gptfouro
& 92.38
& 81.13
& 86.71
& 72.83
& 64.87
& 76.38
& 72.02
& 74.20 \\

\rowcolor[gray]{0.92}
Gemini 3 Flash
& 95.61
& 90.49
& 92.46
& 78.66
& 78.86
& 85.12
& 83.04
& 84.08 \\

\rowcolor[gray]{0.92}
Gemini 3.1 Pro 
& 95.77
& 81.68
& 82.84
& 73.33
& 73.98
& 77.96
& 81.73
& 79.85 \\

\rowcolor[gray]{0.92} 
Claude Sonnet 4.6 
& 97.11
& 91.89
& 94.17
& 68.53
& 66.35
& 80.23
& 80.73
& 80.48 \\

\rowcolor[gray]{0.92}
Claude Opus 4.6 
& 95.05
& 90.20
& 92.01
& 73.10
& 69.13
& 81.11
& 79.68
& 80.40 \\

\bottomrule
\end{tabular}
