# Supplementary material for: PrismaCoder: Pushing the Boundaries of Open Multimodal Code Intelligence through Decomposed Rubric Synthesis
Source: arXiv:2610.20538 source file (2026-10-14)
Supplement: Supplementary file 6 [file chemdraw.tex]

\setlength{\tabcolsep}{7pt}
\caption{ChemDraw, full metrics on the 128-sample test set. Tani.\,(mean) averages over
RDKit-valid outputs; the other columns count all samples. }
\label{tab:chemdraw}
\begin{tabular}{l ccccc}
\toprule
Model & Valid. & \makecell{Exact\\Match} & \makecell{Tani.\\(mean)} & \makecell{Tani.\\$=1$} & \makecell{Tani.\\$\geq.85$} \\
\midrule
\multicolumn{6}{l}{\textit{Open models}} \\
Qwen3-VL-8B-Instruct & 78.91\% & 25.00\% & 54.79 & 25.00\% & 25.00\% \\
Qwen3-VL-30B-A3B-Instruct & 82.03\% & 26.56\% & 54.55 & 27.34\% & 28.12\% \\
Qwen3.5-9B & 88.28\% & 33.59\% & 66.79 & 37.50\% & 39.84\% \\
Qwen3.5-35B-A3B & 92.97\% & 53.12\% & 79.86 & 57.81\% & 60.16\% \\
\rowcolor{boxblue} \textbf{\modelnine} & 96.88\% & 83.59\% & 95.94 & 87.50\% & 89.06\% \\
\rowcolor{boxblue} \textbf{\modelthirtyfive} & 100.00\% & 92.19\% & 97.56 & 95.31\% & 95.31\% \\
\midrule
\multicolumn{6}{l}{\textit{Proprietary}} \\
\rowcolor[gray]{0.92} \gptfouro & 92.19\% & 32.03\% & 57.80 & 33.59\% & 33.59\% \\
\rowcolor[gray]{0.92} Gemini 3 Flash & 63.28\% & 52.34\% & 81.39 & 53.12\% & 53.91\% \\
\rowcolor[gray]{0.92} Claude Sonnet 4.6 & 88.28\% & 53.91\% & 85.43 & 61.72\% & 64.06\% \\
\rowcolor[gray]{0.92} Claude Opus 4.6 & 96.88\% & 52.34\% & 77.71 & 56.25\% & 57.81\% \\
\rowcolor[gray]{0.92} Kimi K2.5 & 91.41\% & 65.62\% & 91.20 & 75.00\% & 76.56\% \\
\bottomrule
\end{tabular}
