# Supplementary material for: PrismaCoder: Pushing the Boundaries of Open Multimodal Code Intelligence through Decomposed Rubric Synthesis
Source: arXiv:2610.20538 source file (2026-10-14)
Supplement: Supplementary file 7 [file data-source.tex]

\begin{table}[htbp]
\centering
\caption{Data sources and routing statistics.}
\label{tab:data_source_stat}
\resizebox{\linewidth}{!}{
\begin{tabular}{lrrr}
\toprule
\textbf{Data Source} &
\textbf{\# Seed Samples} &
\textbf{\# Regenerated Samples} &
\textbf{\# Synthesized Samples} \\
\midrule
MCD dataset
    & 598,000 & 307,184 & 273,199 \\
GitHub repositories
    & 417,000 & 297,942 & 188,630 \\
WebCode2M (Generate)
    & 243,100 & 182,300 & 215,663 \\
WebCode2M (Edit)
    & 264,541 & 167,810 & 190,882 \\
JanusCoder-800K
    & 109,826 & 80,000 & 29,000 \\
WebSight
    & 1,922,671 & 40,000 & 12,000 \\
ProImageBench
    & 654 & 600 & 80 \\
MMMG
    & 4456 & 2400 & 975 \\
UniSVG
    & 528,591 & 65,100 & 51,100 \\
OmniSVG
    & 255,412 & 37,000 & 10,000 \\
arXiv papers
    & 67,000 & 60,155 & 21,400 \\
PubChem
    & 60,000 & 60,000 & 59,000 \\
Manim video code
    & 41,707 & 25,440 & 16,300 \\
\bottomrule
\end{tabular}
}
\end{table}
