# Supplementary material for: PrismaCoder: Pushing the Boundaries of Open Multimodal Code Intelligence through Decomposed Rubric Synthesis
Source: arXiv:2610.20538 source file (2026-10-14)
Supplement: Supplementary file 8 [file design2code.tex]

\setlength{\tabcolsep}{3pt}
\caption{Design2Code, full metrics.}
\label{tab:design2code}
\resizebox{\linewidth}{!}{%
\begin{tabular}{l ccccccc}
\toprule
Model & Block & Text & Pos. & Color & CLIP & Avg & \makecell{LLM\\Score} \\
\midrule
\multicolumn{8}{l}{\textit{Open models}} \\
JanusCoderV-7B & 63.88 & 85.40 & 62.74 & 59.11 & 82.94 & 70.81 & 36.49 \\
JanusCoderV-8B & 59.11 & 81.72 & 61.45 & 57.63 & 83.13 & 68.61 & 34.53 \\
VinciCoder-7B & 71.01 & 87.30 & 68.04 & 71.28 & 85.58 & 76.64 & 42.30 \\
VinciCoder-8B & 79.41 & 91.79 & 73.90 & 77.00 & 87.37 & 81.89 & 45.72 \\
\rowcolor{boxblue} \textbf{\modelnine} & \textbf{90.09} & \textbf{95.95} & \textbf{89.30} & \underline{90.00} & \textbf{92.37} & \textbf{91.54} & \textbf{70.51} \\
\rowcolor{boxblue} \textbf{\modelthirtyfive} & \underline{89.45} & \underline{95.47} & \underline{89.14} & \textbf{90.05} & \underline{91.98} & \underline{91.22} & \underline{67.55} \\
\midrule
\multicolumn{8}{l}{\textit{Proprietary}} \\
\rowcolor[gray]{0.92} \gptfouro & 89.50 & 96.91 & 83.67 & 82.27 & 88.80 & 88.23 & 58.48 \\
\rowcolor[gray]{0.92} Gemini 3.1 Pro & 90.55 & 95.21 & 88.58 & 87.69 & 91.46 & 90.70 & 70.90 \\
\bottomrule
\end{tabular}
}
