# Supplementary material for: PrismaCoder: Pushing the Boundaries of Open Multimodal Code Intelligence through Decomposed Rubric Synthesis
Source: arXiv:2610.20538 source file (2026-10-14)
Supplement: Supplementary file 9 [file designbench.tex]

\setlength{\tabcolsep}{4pt}
\caption{DesignBench, full metrics for generation and editing.}
\label{tab:designbench-full}
\begin{tabular}{l cccc cccc}
\toprule
& \multicolumn{4}{c}{Generation} & \multicolumn{4}{c}{Editing} \\
\cmidrule(lr){2-5}\cmidrule(lr){6-9}
Model & Judge & CLIP & MAE$\downarrow$ & SSIM & Judge & CMS & MAE$\downarrow$ & SSIM \\
\midrule
\multicolumn{9}{l}{\textit{Open models}} \\
JanusCoderV-7B & 40.37 & 71.34 & 77.05 & 0.5910 & 7.44 & 0.2234 & 30.11 & 0.8399 \\
JanusCoderV-8B & 34.30 & 68.38 & 83.64 & 0.5822 & 7.26 & 0.2346 & 28.57 & 0.8446 \\
VinciCoder-7B & 43.24 & 72.81 & 68.05 & 0.6137 & 1.40 & 0.1686 & 45.33 & 0.8119 \\
VinciCoder-8B & 48.09 & 76.79 & 61.86 & 0.6330 & 1.71 & 0.1514 & 41.83 & 0.8199 \\
\rowcolor{boxblue} \textbf{\modelnine} & \textbf{69.95} & \textbf{84.77} & \underline{42.07} & \underline{0.6956} & \textbf{8.93} & \textbf{0.2791} & \textbf{30.56} & \underline{0.8373} \\
\rowcolor{boxblue} \textbf{\modelthirtyfive} & \underline{68.98} & \underline{84.56} & \textbf{41.97} & \textbf{0.6972} & \underline{8.89} & \underline{0.2601} & \underline{30.67} & \textbf{0.8398} \\
\midrule
\multicolumn{9}{l}{\textit{Proprietary}} \\
\rowcolor[gray]{0.92} \gptfouro & 52.64 & 76.45 & 64.11 & 0.6259 & 8.89 & 0.3567 & 27.97 & 0.8439 \\
\rowcolor[gray]{0.92} Gemini 3.1 Pro & 69.47 & 85.23 & 44.11 & 0.6914 & 9.57 & 0.3751 & 26.13 & 0.8548 \\
\bottomrule
\end{tabular}
