# Supplementary material for: PrismaCoder: Pushing the Boundaries of Open Multimodal Code Intelligence through Decomposed Rubric Synthesis
Source: arXiv:2610.20538 source file (2026-10-14)
Supplement: Supplementary file 11 [file interactscience.tex]

\setlength{\tabcolsep}{4pt}
\caption{InteractScience, full metrics for both lenses. }
\label{tab:interactscience}
\resizebox{\linewidth}{!}{%
\begin{tabular}{l ccc c}
\toprule
& \multicolumn{3}{c}{PFT} & VQT \\
\cmidrule(lr){2-4}\cmidrule(lr){5-5}
Model & Overall & Avg. & Perfect & VLM \\
\midrule
JanusCoderV-7B & 17.73\% & 16.91\% & 4.20\% & 27.67 \\
JanusCoderV-8B & 17.60\% & 17.30\% & 4.20\% & 33.32 \\
VinciCoder-7B & 0.40\% & 0.00\% & 0.00\% & 0.00 \\
VinciCoder-8B & 0.40\% & 0.42\% & 0.00\% & 2.33 \\
\rowcolor{boxblue} \textbf{\modelnine}       & 24.80\% & 22.47\% & 7.69\% & 51.87 \\
\rowcolor{boxblue} \textbf{\modelthirtyfive} & 28.00\% & 25.94\% & 6.99\% & 53.54 \\
\rowcolor[gray]{0.92} \gptfouro & 31.07\% & 28.59\% & 10.49\% & 46.01 \\
\bottomrule
\end{tabular}}
