# Supplementary material for: PrismaCoder: Pushing the Boundaries of Open Multimodal Code Intelligence through Decomposed Rubric Synthesis
Source: arXiv:2610.20538 source file (2026-10-14)
Supplement: Supplementary file 12 [file pandasplotbench.tex]

\setlength{\tabcolsep}{4pt}
\caption{PandasPlotBench, full metrics under the Visual and Task lenses.
}
\label{tab:pandasplot-full}

\begin{tabular}{l c cc cc}
\toprule
& \makecell{Incorr.\\Code$\downarrow$}
& \multicolumn{2}{c}{Mean}
& \multicolumn{2}{c}{Good $\geq$75} \\
\cmidrule(lr){3-4}\cmidrule(lr){5-6}
Model & & Vis. & Task & Vis. & Task \\
\midrule

Qwen3-VL-8B-Instruct
    & 16.00\% & 60.01 & 73.67 & 0.506 & 0.701 \\
Qwen3-VL-30B-A3B-Instruct
    & 11.43\% & 60.05 & 80.58 & 0.555 & 0.806 \\

Qwen3.5-9B
    & 24.57\% & 52.98 & 65.47 & 0.417 & 0.640 \\
Qwen3.5-35B-A3B
    & 15.43\% & 60.36 & 75.17 & 0.509 & 0.743 \\

JanusCoderV-7B
    & 23.43\% & 53.05 & 65.77 & 0.440 & 0.640 \\
JanusCoderV-8B
    & 26.30\% & 56.30 & 70.91 & 0.450 & 0.650 \\

VinciCoder-7B
    & 9.14\% & 25.37 & 51.57 & 0.137 & 0.314 \\
VisCoder2-7B
    & 20.00\% & 59.48 & 67.59 & 0.511 & 0.623 \\

\rowcolor{boxblue}
\textbf{PrismaCoder-9B}
    & 10.29\%
    & 60.54
    & 77.94
    & 0.497
    & 0.766 \\

\rowcolor{boxblue}
\textbf{PrismaCoder-35B}
    & 9.29\% & {62.38} & 79.85 & 0.606 & 0.772 \\

\midrule

\rowcolor[gray]{0.92}
GPT-4o
    & 8.00\% & 67.63 & 82.46 & 0.571 & 0.822 \\
\rowcolor[gray]{0.92}
Gemini 3 Flash
    & 3.43\% & 69.95 & 91.21 & 0.566 & 0.949 \\
\rowcolor[gray]{0.92}
Gemini 3.1 Pro
    & 1.71\% & 78.41 & 94.70 & 0.703 & 0.960 \\
\rowcolor[gray]{0.92}
Claude Sonnet 4.6
    & 3.43\% & 74.59 & 91.93 & 0.686 & 0.914 \\
\rowcolor[gray]{0.92}
Claude Opus 4.6
    & 1.71\% & 76.03 & 94.97 & 0.674 & 0.966 \\

\bottomrule
\end{tabular}
