# Supplementary material for: PrismaCoder: Pushing the Boundaries of Open Multimodal Code Intelligence through Decomposed Rubric Synthesis
Source: arXiv:2610.20538 source file (2026-10-14)
Supplement: Supplementary file 13 [file reward_spec.tex]

\begin{table}[h]
\centering
\footnotesize
\caption{RL rewards by task family. Rewards lie in $[0,1]$;
unscoreable completions receive $0$.}
\label{tab:reward-spec}
\setlength{\tabcolsep}{4pt}
\begin{tabular}{l l l l}
\toprule
Task family & Spec.\ $\to$ output & Reward Type & Weights Assignment \\
\midrule
Chart generation & text $\to$ Python & Rubrics & $\lambda_c=\lambda_v = 0.5$ \\
Chart reproduction & image $\to$ Python & Rubrics & $\lambda_c=\lambda_v = 0.5$ \\
Webpage generation & text $\to$ HTML & Rubrics & $\lambda_c=0.4, \lambda_v = 0.6$ \\
HTML demonstration & plan $\to$ HTML & Rubrics & $\lambda_c=0.4, \lambda_v = 0.6$ \\
\quad + reference snapshots & plan + images $\to$ HTML & Rubrics & $\lambda_c=0.4, \lambda_v = 0.6$ \\
SVG generation & text $\to$ SVG & Rubrics & $\lambda_c=0.4, \lambda_v = 0.6$ \\
Interface reproduction & image $\to$ HTML & Rubrics+Holistic & $\lambda_c=0.2,\lambda_v = 0.5, \lambda_h = 0.3$ \\
SVG reproduction & image $\to$ SVG & Rubrics+Holistic & $\lambda_c=0.2,\lambda_v = 0.5, \lambda_h = 0.3$ \\
Interface editing & page + instr.\ $\to$ HTML & Rubrics+Holistic & $\lambda_c=0.2,\lambda_v = 0.4, \lambda_h = 0.4$ \\
\bottomrule
\end{tabular}
\end{table}
