# Supplementary material for: PrismaCoder: Pushing the Boundaries of Open Multimodal Code Intelligence through Decomposed Rubric Synthesis
Source: arXiv:2610.20538 source file (2026-10-14)
Supplement: Supplementary file 14 [file unisvg.tex]

\setlength{\tabcolsep}{4pt}
\caption{Full UniSVG metrics~\citep{li2025unisvg}.}
\label{tab:unisvg}
\resizebox{\linewidth}{!}{%
\begin{tabular}{l ccc}
\toprule
Model & ISVGen & TSVGen & Final \\
\midrule
JanusCoderV-7B & 61.60 & 66.43 & 61.23 \\
JanusCoderV-8B  & 62.47 & 67.28 & 63.47 \\
VinciCoder-7B & 85.72 & 64.06 & 67.22 \\
VinciCoder-8B & 87.18 & 63.45 & 67.58 \\
\rowcolor{boxblue} \textbf{\modelnine} & 69.64 & 68.49 & 65.31 \\
\rowcolor{boxblue} \textbf{\modelthirtyfive} & 84.14 & 70.72 & 72.96 \\
\rowcolor[gray]{0.92} \gptfouro & 70.98 & 72.80 & 69.60 \\
\bottomrule
\end{tabular}}
