# Supplementary material for: PrismaCoder: Pushing the Boundaries of Open Multimodal Code Intelligence through Decomposed Rubric Synthesis
Source: arXiv:2610.20538 source file (2026-10-14)
Supplement: Supplementary file 15 [file visplotbench_avg.tex]

\setlength{\tabcolsep}{4pt}
\caption{VisPlotBench averaged metrics.}
\label{tab:visplot-avg}
\resizebox{\linewidth}{!}{%
\begin{tabular}{l c cc cc}
\toprule
& \makecell{Incorr.\\Code$\downarrow$} & \multicolumn{2}{c}{Mean} & \multicolumn{2}{c}{Good $\geq$75} \\
\cmidrule(lr){3-4}\cmidrule(lr){5-6}
Model & & Vis. & Task & Vis. & Task \\
\midrule
VinciCoder-7B    & 35.90\% & 15.93 & 23.95 & 4.16 & 10.11 \\
VinciCoder-8B    & 36.08\% & 8.84 & 12.55 & 1.50 & 2.80 \\
\rowcolor{boxblue} \textbf{\modelnine}       & 34.70\% & 36.40 & 53.99 & 23.12 & 52.62 \\
\rowcolor{boxblue} \textbf{\modelthirtyfive} & 28.86\% & 45.16 & 62.47 & 32.55 & 61.49 \\
\rowcolor[gray]{0.92} \gptfouro & 32.01\% & 38.19 & 56.01 & 24.75 & 52.75 \\
\bottomrule
\end{tabular}}
