# Supplementary material for: PrismaCoder: Pushing the Boundaries of Open Multimodal Code Intelligence through Decomposed Rubric Synthesis
Source: arXiv:2610.20538 source file (2026-10-14)
Supplement: Supplementary file 16 [file visplotbench_languages.tex]

\setlength{\tabcolsep}{4pt}
\caption{VisPlotBench, per-language incorrect-code rate. }
\label{tab:visplot-full}
\resizebox{\linewidth}{!}{%
\begin{tabular}{l c cccccccc}
\toprule
\rowcolor{boxredlight}
Model & \makecell{Avg.\\Incorr.$\downarrow$}
& Python & \makecell{Vega-\\Lite} & LilyPond & Mermaid & SVG & \LaTeX & \makecell{Asym-\\ptote} & HTML \\
\midrule
\multicolumn{10}{l}{\emph{Open models}} \\
VinciCoder-7B    & 35.90\% & 10.20\% & 66.67\% & 100.00\% & 7.63\% & 1.54\% & 56.25\% & 21.74\% & 23.15\% \\
VinciCoder-8B    & 36.08\% & 2.55\% & 57.36\% & 100.00\% & 4.58\% & 7.69\% & 58.93\% & 19.57\% & 37.96\% \\
VisCoder2        & 33.26\% & 43.37\% & 16.28\% & 41.82\% & 25.95\% & 12.31\% & 61.61\% & 43.48\% & 21.30\% \\
\rowcolor{boxblue} \textbf{\modelnine}       & 34.70\% & 29.59\% & 13.18\% & 85.45\% & 12.21\% & 1.54\% & 66.96\% & 65.22\% & 19.44\% \\
\rowcolor{boxblue} \textbf{\modelthirtyfive} & 28.86\% & 11.22\% & 3.88\% & 89.09\% & 9.92\% & 0.00\% & 70.54\% & 51.09\% & 11.11\% \\
\midrule
\multicolumn{10}{l}{\emph{Proprietary}} \\
\rowcolor[gray]{0.92} \gptfouro & 32.01\% & 22.45\% & 8.53\% & 40.00\% & 24.43\% & 0.00\% & 61.61\% & 75.00\% & 24.07\% \\
\bottomrule
\end{tabular}}
