# Supplementary material for: PrismaCoder: Pushing the Boundaries of Open Multimodal Code Intelligence through Decomposed Rubric Synthesis
Source: arXiv:2610.20538 source file (2026-10-14)
Supplement: Supplementary file 17 [file webcode2m.tex]

\setlength{\tabcolsep}{3pt}
\caption{WebCode2M, full metrics by code length.}
\label{tab:webcode2m-full}
\resizebox{\linewidth}{!}{%
\begin{tabular}{l cccc cccc cccc cccc}
\toprule
& \multicolumn{4}{c}{Short} & \multicolumn{4}{c}{Mid} & \multicolumn{4}{c}{Long} & \multicolumn{4}{c}{Average} \\
\cmidrule(lr){2-5}\cmidrule(lr){6-9}\cmidrule(lr){10-13}\cmidrule(lr){14-17}
Model
& LLM & Visual & CLIP & \makecell{Tree-\\BLEU}
& LLM & Visual & CLIP & \makecell{Tree-\\BLEU}
& LLM & Visual & CLIP & \makecell{Tree-\\BLEU}
& LLM & Visual & CLIP & \makecell{Tree-\\BLEU} \\
\midrule
\multicolumn{17}{l}{\textit{Open models}} \\
JanusCoderV-7B & 40.10 & 72.39 & 76.11 & 29.64 & 43.06 & 74.08 & 76.77 & \underline{37.43} & 39.61 & 72.24 & 75.11 & \textbf{39.37} & 40.92 & 72.90 & 76.00 & \textbf{35.48}  \\
JanusCoderV-8B & 34.60 & 65.74 & 73.14 & \underline{30.37} & 36.17 & 65.41 & 73.46 & 29.88 & 34.74 & 66.71 & 72.53 & 27.66 & 35.17 & 65.95 & 73.04 & 29.30  \\
VinciCoder-7B & 46.01 & 76.76 & 80.43 & 30.00 & 44.34 & 73.57 & 79.38 & \textbf{38.11} & 38.99 & 66.92 & 75.97 & 29.74 & 43.11 & 72.42 & 78.59 & 32.62 \\
VinciCoder-8B & 48.35 & 80.43 & 82.03 & \textbf{31.39} & 48.08 & 79.53 & 81.70 & \textbf{39.48} & 42.05 & 74.83 & 78.63 & \underline{32.57} & 46.16 & 78.26 & 80.79 & \underline{34.48}  \\
\rowcolor{boxblue} \textbf{\modelnine} & \textbf{70.65} & \textbf{90.06} & \textbf{90.29} & 17.23 & \textbf{69.08} & \textbf{90.02} & \textbf{87.76} & 18.65 & \textbf{69.42} & \textbf{91.15} & \textbf{87.32} & 17.23 & \textbf{69.72} & \textbf{90.41} & \textbf{88.46} & 17.70  \\
\rowcolor{boxblue} \textbf{\modelthirtyfive} & \underline{68.52} & \underline{89.58} & \underline{89.93} & 15.78 & \underline{68.12} & \underline{89.54} & \underline{87.21} & 17.77 & \underline{66.69} & \underline{89.87} & \underline{86.19} & 17.18 & \underline{67.78} & \underline{89.66} & \underline{87.78} & 16.91  \\
\midrule
\multicolumn{17}{l}{\textit{Proprietary}} \\
\rowcolor[gray]{0.92} \gptfouro & 57.62 & 83.96 & 82.10 & 11.73 & 53.27 & 83.35 & 79.62 & 10.00 & 53.93 & 83.03 & 78.94 & 8.13 & 54.94 & 83.45 & 80.22 & 9.95  \\
\rowcolor[gray]{0.92} Gemini 3.1 Pro & 71.67 & 89.23 & 88.52 & 16.77 & 70.83 & 89.78 & 87.58 & 16.56 & 70.40 & 90.87 & 86.82 & 14.44 & 70.97 & 89.96 & 87.64 & 15.92  \\
\bottomrule
\end{tabular}}
